# Supplementary material for: One-shot Transfer Learning for Population Mapping
Source: arXiv:2108.06228 source file (2021-08-17)
Supplement: Supplementary file 1 [file Sec6_supplementary.tex]

%!TEX root = head.tex
\section{APPENDIX FOR REPRODUCIBILITY}\label{sec:Appe}
\subsection{Detailed Settings of Baselines}
We list the detailed setting of baselines in this paper below:
\begin{itemize}
    \item \textbf{UrbanFM:} We use the recommended hyper-parameters (Base Channels=$128$, Residual Blocks=$16$) from official implementation\footnote{https://github.com/yoshall/UrbanFM}. In tasks where UrbanFM needs to accept sequential input with length $L$, we change the input channels to $L$.
    \item \textbf{DeepDPM:} We use $log_{2}N$ resblocks in CNN part, where $N$ is the up-scaling factor and we use 64, 32, and 1 number of feature maps, 9,1,5 as kernel size in each layer.
    \item \textbf{RCAN:} Following the official implementation\footnote{https://github.com/yulunzhang/RCAN}, we use the recommended hyper-parameters: number of features is 64, residual groups is set as 5, residual blocks is set as 10, kernel size is 3, reduction is 16. The number of input channels is also changed to $L$ due to the requirement of the sequential input.
    \item \textbf{DBPN:} We use the recommended hyper-parameters of DBPN from the official implementation\footnote{https://github.com/alterzero/DBPN-Pytorch}. For $\times2$ task, the number of layers is $7$, kernel size is $6$, stride is $2$, padding is $2$. For $\times4$ task, the number of layers is $7$, kernel size is $8$, stride is $4$, padding is $2$. While the number of input channels is also changed by length of sequential input $L$.
    \item \textbf{RRN:} Firstly, we use a 3D convolution with time stride=$8$ to simplify the input sequential maps. With the simplified feature maps, we follow the recommended parameters in official implementation\footnote{https://github.com/junpan19/RRN}.
    \item \textbf{RBPN:} We also employ a 3D convolution with time stride=8 to simplify the input sequential maps. With the simplified feature maps, we follow the official implementation\footnote{https://github.com/alterzero/RBPN-PyTorch}.
\end{itemize}

\begin{table*}[htbp]
\resizebox{1.0\textwidth}{!}{
\begin{tabular}{c||ccccc||ccccc||ccccc||ccccc}
\toprule
\textbf{Target Domain} & \multicolumn{5}{c||}{\textbf{CITY2 (X2) (Cross Cities)}}                                     & \multicolumn{5}{c||}{\textbf{CITY2 (X4) (Cross Cities)}}                                     & \multicolumn{5}{c||}{\textbf{CITY2 (X8) (Cross Cities)}}                                     & \multicolumn{5}{c}{\textbf{CITY2 (Cross Granularities)}}                                   \\ \hline
\textbf{Metrics}       & \textbf{RMSE}    & \textbf{NRMSE}   & \textbf{MAE}     & \textbf{MAPE}    & \textbf{CORR}   & \textbf{RMSE}    & \textbf{NRMSE}   & \textbf{MAE}     & \textbf{MAPE}    & \textbf{CORR}   & \textbf{RMSE}    & \textbf{NRMSE}   & \textbf{MAE}     & \textbf{MAPE}    & \textbf{CORR}   & \textbf{RMSE}    & \textbf{NRMSE}   & \textbf{MAE}     & \textbf{MAPE}    & \textbf{CORR}   \\ \midrule
\textbf{Bibubic}       & 19.4627          & 0.4875           & 12.9731          & 0.325            & 0.8735          & 25.8791          & 0.6483           & 17.8487          & 0.4471           & 0.7588          & 29.342           & 0.735            & 20.9715          & 0.5253           & 0.6715          & 19.4627          & 0.4875           & 12.9731          & 0.325            & 0.8735          \\
\textbf{LightGBM}      & 19.507           & 0.4886           & 12.7545          & 0.3195           & 0.8827          & 26.5186          & 0.6643           & 17.8491          & 0.4471           & 0.768           & 30.6536          & 0.7679           & 21.4466          & 0.5372           & 0.6726          & 22.2054          & 0.5562           & 14.0327          & 0.3515           & 0.8523          \\ \midrule
\textbf{DeepDPM}       & 19.9036          & 0.4986           & 13.7373          & 0.3441           & 0.8766          & 25.9132          & 0.6491           & 16.9315          & 0.4241           & 0.7969          & 36.1815          & 0.9063           & 24.3855          & 0.6108           & 0.6199          & 19.6983          & 0.4934           & 13.3138          & 0.3335           & 0.8727          \\
\textbf{UrbanFM}       & 16.546           & 0.4145           & 10.6395          & 0.2665           & 0.9171          & 20.8997          & 0.5235           & 13.4987          & 0.3381           & 0.8659          & 19.8849          & 0.4981           & 12.0833          & 0.3027           & 0.8854          & {\ul 17.6771}    & {\ul 0.4428}     & {\ul 11.219}     & {\ul 0.281}      & {\ul 0.9061}    \\ \midrule
\textbf{RCAN}          & 17.3804          & 0.4354           & 10.8795          & 0.2725           & 0.9107          & 21.6881          & 0.5433           & 14.352           & 0.3595           & 0.8528          & 26.0136          & 0.6516           & 16.6726          & 0.4176           & 0.8291          & 18.6983          & 0.4684           & 12.6933          & 0.318            & 0.8892          \\ 
\textbf{DBPN}          & 17.7453          & 0.4445           & 11.4037          & 0.2857           & 0.9083          & 25.2231          & 0.6318           & 16.1284          & 0.404            & 0.8181          & 28.4906          & 0.7137           & 17.8626          & 0.4474           & 0.7797          & 18.4023          & 0.461            & 12.1017          & 0.3031           & 0.8976          \\ 
\textbf{RRN}           & 17.8356          & 0.4468           & 11.5016          & 0.2881           & 0.905           & 38.977           & 0.9763           & 25.1846          & 0.6309           & 0.6963          & 75.2558          & 1.8851           & 42.1523          & 1.0559           & 0.6149          & 19.1953          & 0.4808           & 13.181           & 0.3302           & 0.8878          \\ 
\textbf{RBPN}          & 17.9094          & 0.4486           & 12.1417          & 0.3041           & 0.9014          & 22.8572          & 0.5726           & 15.6123          & 0.3911           & 0.8345          & 25.8437          & 0.6474           & 17.4959          & 0.4383           & 0.7934          & 21.3816          & 0.5356           & 14.4584          & 0.3622           & 0.8589          \\ \midrule
\textbf{SNet}          & 15.3947          & 0.3856           & 9.4264           & 0.2361           & 0.9295          & 19.4442          & 0.4871           & 12.1049          & 0.3032           & 0.8873          & 21.8873          & 0.5483           & 13.9482          & 0.3494           & 0.8593          &                  &                  &                  &                  &                 \\ 
\textbf{SNet+PGNet}    & 15.0212          & 0.3763           & 9.3888           & 0.2352           & 0.9326          & 17.8802          & 0.4479           & 11.4672          & 0.2872           & 0.9025          & 20.5056          & 0.5137           & 13.6976          & 0.3431           & 0.8678          &                  &                  &                  &                  &                 \\ 
\textbf{STNet}         & 15.0495          & 0.377            & 9.3038           & 0.2331           & 0.9335          & 18.3182          & 0.4589           & 11.1873          & 0.2802           & 0.9015          & 20.6691          & 0.5177           & 12.9792          & 0.3251           & 0.8741          &                  &                  &                  &                  &                 \\ 
\textbf{MAML+STNet}    & 14.9734          & 0.3751           & 9.2698           & 0.2322           & 0.9343          & 18.5612          & 0.4649           & 11.4249          & 0.2862           & 0.8985          & 20.6137          & 0.5164           & 13.0256          & 0.3263           & 0.875           &                  &                  &                  &                  &                 \\ 
\textbf{STNet+PGNet}   & \textbf{14.1569} & \textbf{0.3546}  & \textbf{8.3967}  & \textbf{0.2103}  & \textbf{0.9419} & {\ul 16.7954}    & {\ul 0.4207}     & {\ul 10.336}     & {\ul 0.2589}     & {\ul 0.9162}    & {\ul 18.475}     & {\ul 0.4628}     & {\ul 11.5924}    & {\ul 0.2904}     & {\ul 0.8979}    &                  &                  &                  &                  &                 \\ 
\textbf{PSRNet}        & {\ul 14.7143}    & {\ul 0.3686}     & {\ul 9.0659}     & {\ul 0.2271}     & {\ul 0.9365}    & \textbf{16.7457} & \textbf{0.4195}  & \textbf{10.2143} & \textbf{0.2559}  & \textbf{0.917}  & \textbf{18.2632} & \textbf{0.4575}  & \textbf{11.3176} & \textbf{0.2835}  & \textbf{0.9002} & \textbf{13.0725} & \textbf{0.3275}  & \textbf{7.9503}  & \textbf{0.1991}  & \textbf{0.9498} \\ \hline
\textbf{Improv.}   & \textbf{15.52\%} & \textbf{15.53\%} & \textbf{23.79\%} & \textbf{23.80\%} & \textbf{2.67\%} & \textbf{21.36\%} & \textbf{21.35\%} & \textbf{27.13\%} & \textbf{27.11\%} & \textbf{5.76\%} & \textbf{8.16\%}  & \textbf{8.15\%}  & \textbf{6.34\%}  & \textbf{6.34\%}  & \textbf{1.67\%} & \textbf{26.05\%} & \textbf{26.04\%} & \textbf{29.14\%} & \textbf{29.15\%} & \textbf{4.82\%} \\ \midrule
\textbf{Target Domain} & \multicolumn{5}{c||}{CITY3 (X2) (Cross Cities)}                                              & \multicolumn{5}{c||}{CITY3 (X4) (Cross Cities)}                                              & \multicolumn{5}{c||}{CITY3 (X8) (Cross Cities)}                                              & \multicolumn{5}{c}{CITY3 (Cross Granularities)}                                            \\ \hline
\textbf{Metrics}       & RMSE             & NRMSE            & MAE              & MAPE             & CORR            & RMSE             & NRMSE            & MAE              & MAPE             & CORR            & RMSE             & NRMSE            & MAE              & MAPE             & CORR            & RMSE             & NRMSE            & MAE              & MAPE             & CORR            \\ \midrule
\textbf{Bibubic}       & 37.504           & 0.8386           & 20.4538          & 0.4574           & 0.8499          & 50.4365          & 1.1278           & 28.9777          & 0.648            & 0.7033          & 58.8118          & 1.3151           & 36.3592          & 0.813            & 0.5574          & 37.504 & 0.8386 & 20.4538 & 0.4574 & 0.8499\\ 
\textbf{LightGBM}      & 37.4529          & 0.8375           & 20.0207          & 0.4477           & 0.851           & 50.4601          & 1.1284           & 28.6542          & 0.6407           & 0.7068          & 59.1345          & 1.3223           & 36.5012          & 0.8162           & 0.5586 & 41.8102 & 0.9349 & 21.7992 & 0.4875 & 0.8389\\ \midrule
\textbf{DeepDPM}       & 32.1351          & 0.7186           & 17.2336          & 0.3854           & 0.8995          & 41.5014          & 0.928            & 21.1837          & 0.4737           & 0.8424          & 83.2776          & 1.8622           & 44.09            & 0.9859           & 0.1225          & 19.6983          & 0.4934           & 13.3138          & 0.3335           & 0.8727          \\ 
\textbf{UrbanFM}       & 19.8083          & 0.4429           & 10.5936          & 0.2369           & 0.9581          & 27.7215          & 0.6199           & 13.6535          & 0.3053           & 0.9247          & 28.1453          & 0.6294           & 13.1009          & 0.293            & 0.9269          & {\ul 17.6771}    & {\ul 0.4428}     & {\ul 11.219}     & {\ul 0.281}      & {\ul 0.9061}    \\ \midrule
\textbf{RCAN}          & 33.602           & 0.7514           & 19.2509          & 0.4305           & 0.9299          & 28.7524          & 0.6429           & 16.5762          & 0.3707           & 0.927           & 37.611           & 0.841            & 20.5353          & 0.4592           & 0.9036          & 18.6983          & 0.4684           & 12.6933          & 0.318            & 0.8892          \\ 
\textbf{DBPN}          & 20.4376          & 0.457            & 11.3548          & 0.2539           & 0.9564          & 29.9203          & 0.6691           & 16.965           & 0.3794           & 0.9099          & 36.7159          & 0.821            & 19.1835          & 0.429            & 0.912           & 18.4023          & 0.461            & 12.1017          & 0.3031           & 0.8976          \\ 
\textbf{RRN}           & 34.074           & 0.7619           & 19.5061          & 0.4362           & 0.8996          & 50.0075          & 1.1182           & 31.8315          & 0.7118           & 0.7975          & 60.4927          & 1.3527           & 39.6025          & 0.8856           & 0.6695          & 19.1953          & 0.4808           & 13.181           & 0.3302           & 0.8878          \\ 
\textbf{RBPN}          & 23.0956          & 0.5164           & 14.5866          & 0.3262           & 0.9455          & 31.628           & 0.7072           & 19.1963          & 0.4293           & 0.9017          & 37.2798          & 0.8336           & 21.7895          & 0.4872           & 0.885           & 21.3816          & 0.5356           & 14.4584          & 0.3622           & 0.8589          \\ \midrule
\textbf{SNet}          & 18.589           & 0.4157           & 9.2011           & 0.2057           & 0.9633          & 26.1566          & 0.5849           & 12.616           & 0.2821           & 0.9338          & 29.6549          & 0.6631           & 15.2691          & 0.3414           & 0.9131          &                  &                  &                  &                  &                 \\ 
\textbf{SNet+PGNet}    & 17.7402          & 0.3967           & 9.1582           & 0.2048           & 0.966           & 22.4887          & 0.5029           & 11.3496          & 0.2538           & 0.9451          & 26.4319          & 0.5911           & 13.7562          & 0.3076           & 0.9244          &                  &                  &                  &                  &                 \\ 
\textbf{STNet}         & 18.2639          & 0.4084           & 9.1487           & 0.2046           & 0.9661          & 25.5308          & 0.5709           & 12.3324          & 0.2758           & 0.9378          & 29.2517          & 0.6541           & 13.9956          & 0.313            & 0.9257          &                  &                  &                  &                  &                 \\ 
\textbf{MAML+STNet}    & 17.9678          & 0.4018           & 8.9567           & 0.2003           & 0.9667          & 25.8606          & 0.5783           & 12.4289          & 0.2779           & 0.9359          & 29.4891          & 0.6594           & 13.9879          & 0.3128           & 0.9256          &                  &                  &                  &                  &                 \\ 
\textbf{STNet+PGNet}   & {\ul 16.4204}    & {\ul 0.3672}     & {\ul 8.451}      & {\ul 0.189}      & {\ul 0.9713}    & {\ul 21.02}      & {\ul 0.47}       & {\ul 10.3915}    & {\ul 0.2324}     & {\ul 0.9515}    & {\ul 23.9502}    & {\ul 0.5356}     & {\ul 11.9887}    & {\ul 0.2681}     & {\ul 0.9382}    &                  &                  &                  &                  &                 \\ 
\textbf{PSRNet}        & \textbf{16.1735} & \textbf{0.3617}  & \textbf{8.2468}  & \textbf{0.1844}  & \textbf{0.9717} & \textbf{20.8606} & \textbf{0.4665}  & \textbf{10.2796} & \textbf{0.2299}  & \textbf{0.9518} & \textbf{23.8056} & \textbf{0.5323}  & \textbf{11.7768} & \textbf{0.2633}  & \textbf{0.9391} & \textbf{13.0725} & \textbf{0.3275}  & \textbf{7.9503}  & \textbf{0.1991}  & \textbf{0.9498} \\ \hline
\textbf{Improv.}   & \textbf{19.55\%} & \textbf{19.53\%} & \textbf{25.51\%} & \textbf{25.52\%} & \textbf{1.41\%} & \textbf{26.23\%} & \textbf{26.23\%} & \textbf{26.74\%} & \textbf{26.73\%} & \textbf{2.66\%} & \textbf{15.42\%} & \textbf{15.43\%} & \textbf{10.11\%} & \textbf{10.14\%} & \textbf{1.32\%} & \textbf{26.05\%} & \textbf{26.04\%} & \textbf{29.14\%} & \textbf{29.15\%} & \textbf{4.82\%} \\ \bottomrule
\end{tabular}}
\caption{Performance of variants of \OurModel and baselines. Left $3$ columns present the experiments of the cross-cities scenario while rightest column shows the cross-granularities scenario. \textbf{Bold} denotes best (lowest) results and {\ul underline} denotes the second-best results.}
\label{table:complete}
\vspace{-1.0cm}
\end{table*}

\subsection{Hyper-parameters Study and Discussions}
Here, we discuss the implementation and hyper-parameters of \PSRNet in detail. We investigate the effect of 2 influential hyper-parameters from \STNetns: the length of input map sequence and the time stride of 3D convolution. We also investigate 2 hyper-parameters in \PGNetns, which are used to balance 2 trade-offs in \PGNetns. Finally, we investigate the relation between memory-usage and NRMSE of different models to compare the complexity of models.

\subsubsection{Hyper-parameters Study of \emph{\STNetns}}
%In order to research the effect of hyper-parameters, which may have a significant influence on the result of \PSRNetns, 
We conduct a series experiments about 2 hyper-parameters from \STNetns: length of the sequence of input coarse-grained population map (L) and time-stride (TS) of 3D convolution in \OurTSRModelNoSpace. Figure~\ref{fig:frame_stride} shows the performance of \STNet in one-shot transfer learning in $\times2$ and $\times4$ tasks in CITY2 and CITY3 with different lengths of input and time strides. To reduce the influence of other variables, we only employ 1 reference population map to fine-tune these pre-trained \STNetns, rather than employ augmented population maps generated by \PGNetns. Note that for \STNetns, the number of dense layers is determined by length of the input sequence (L) and time stride (TS), that is, the number of layers = L/TS. According to Figure~\ref{fig:frame_stride}, with a longer input sequence of coarse-grained population maps, which provide more spatial-temporal information, our \PSRNet could usually perform better. Besides, to reduce the consumption of \PSRNetns, we employ a 3D convolution with time stride (TS) to simplify the input sequential maps. Therefore, with a shorter stride, \PSRNet usually performs better but it also saves parameters.
\begin{figure}[htbp]
    \subfigure[$\times2$ performance in CITY2.]{
        \includegraphics*[width=0.22\textwidth]{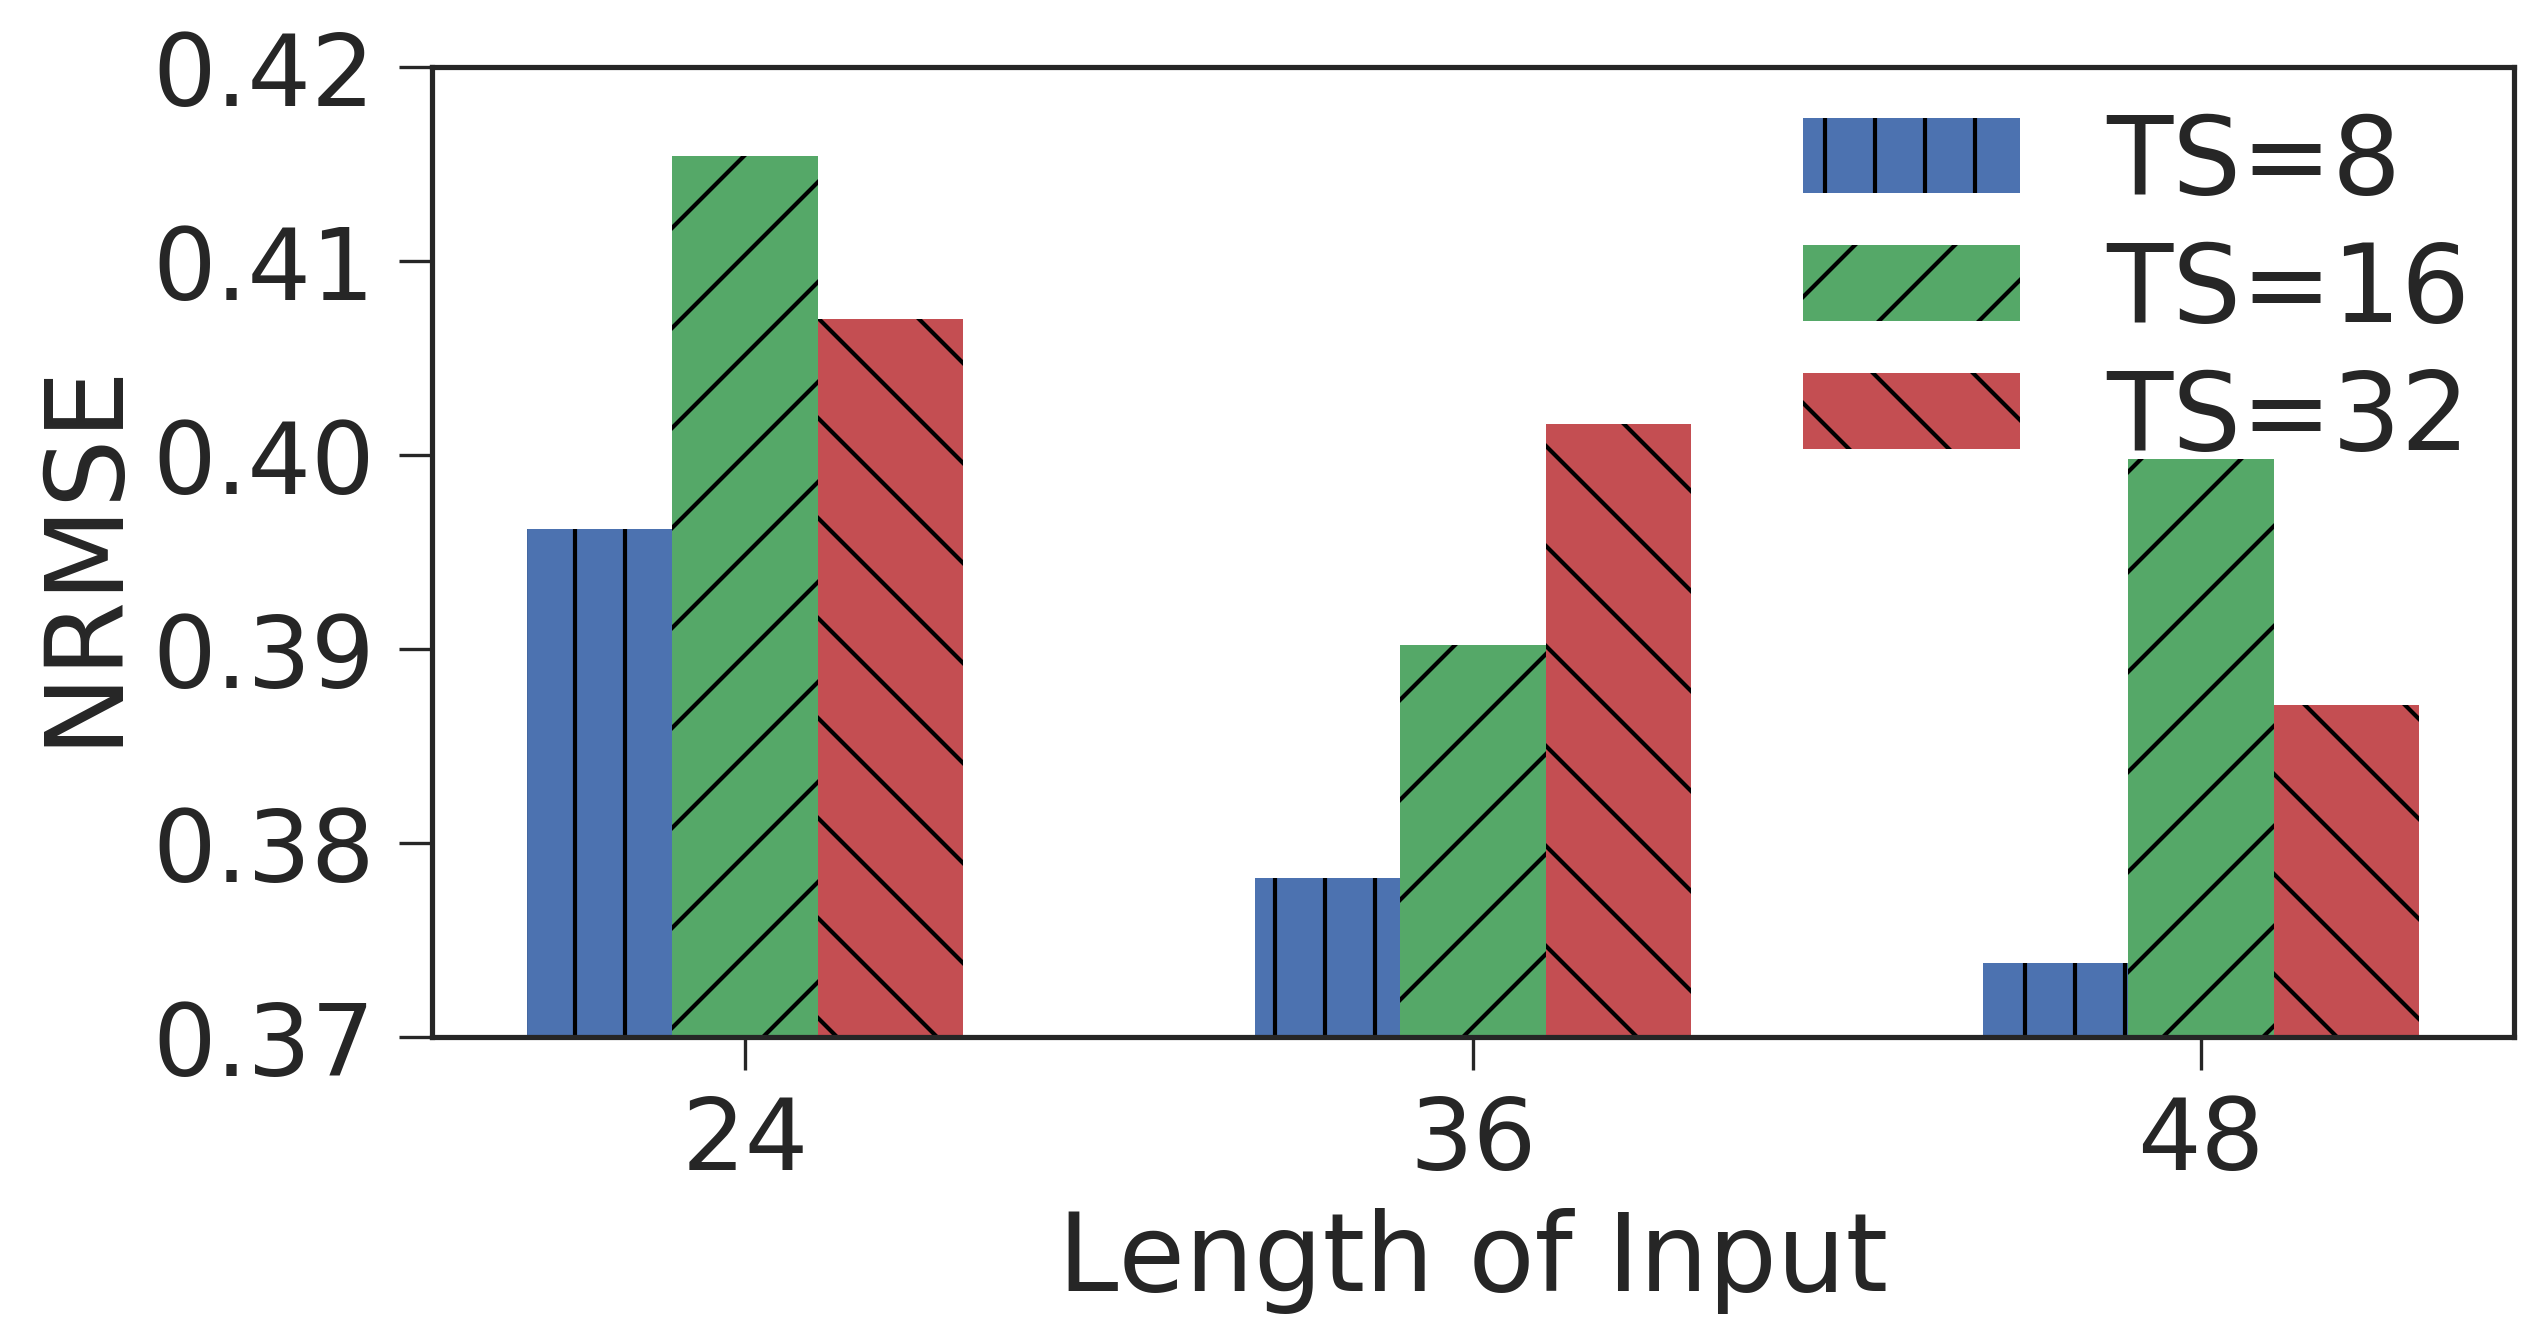}}
    \subfigure[$\times4$ performance in CITY2.]{
        \includegraphics*[width=0.22\textwidth]{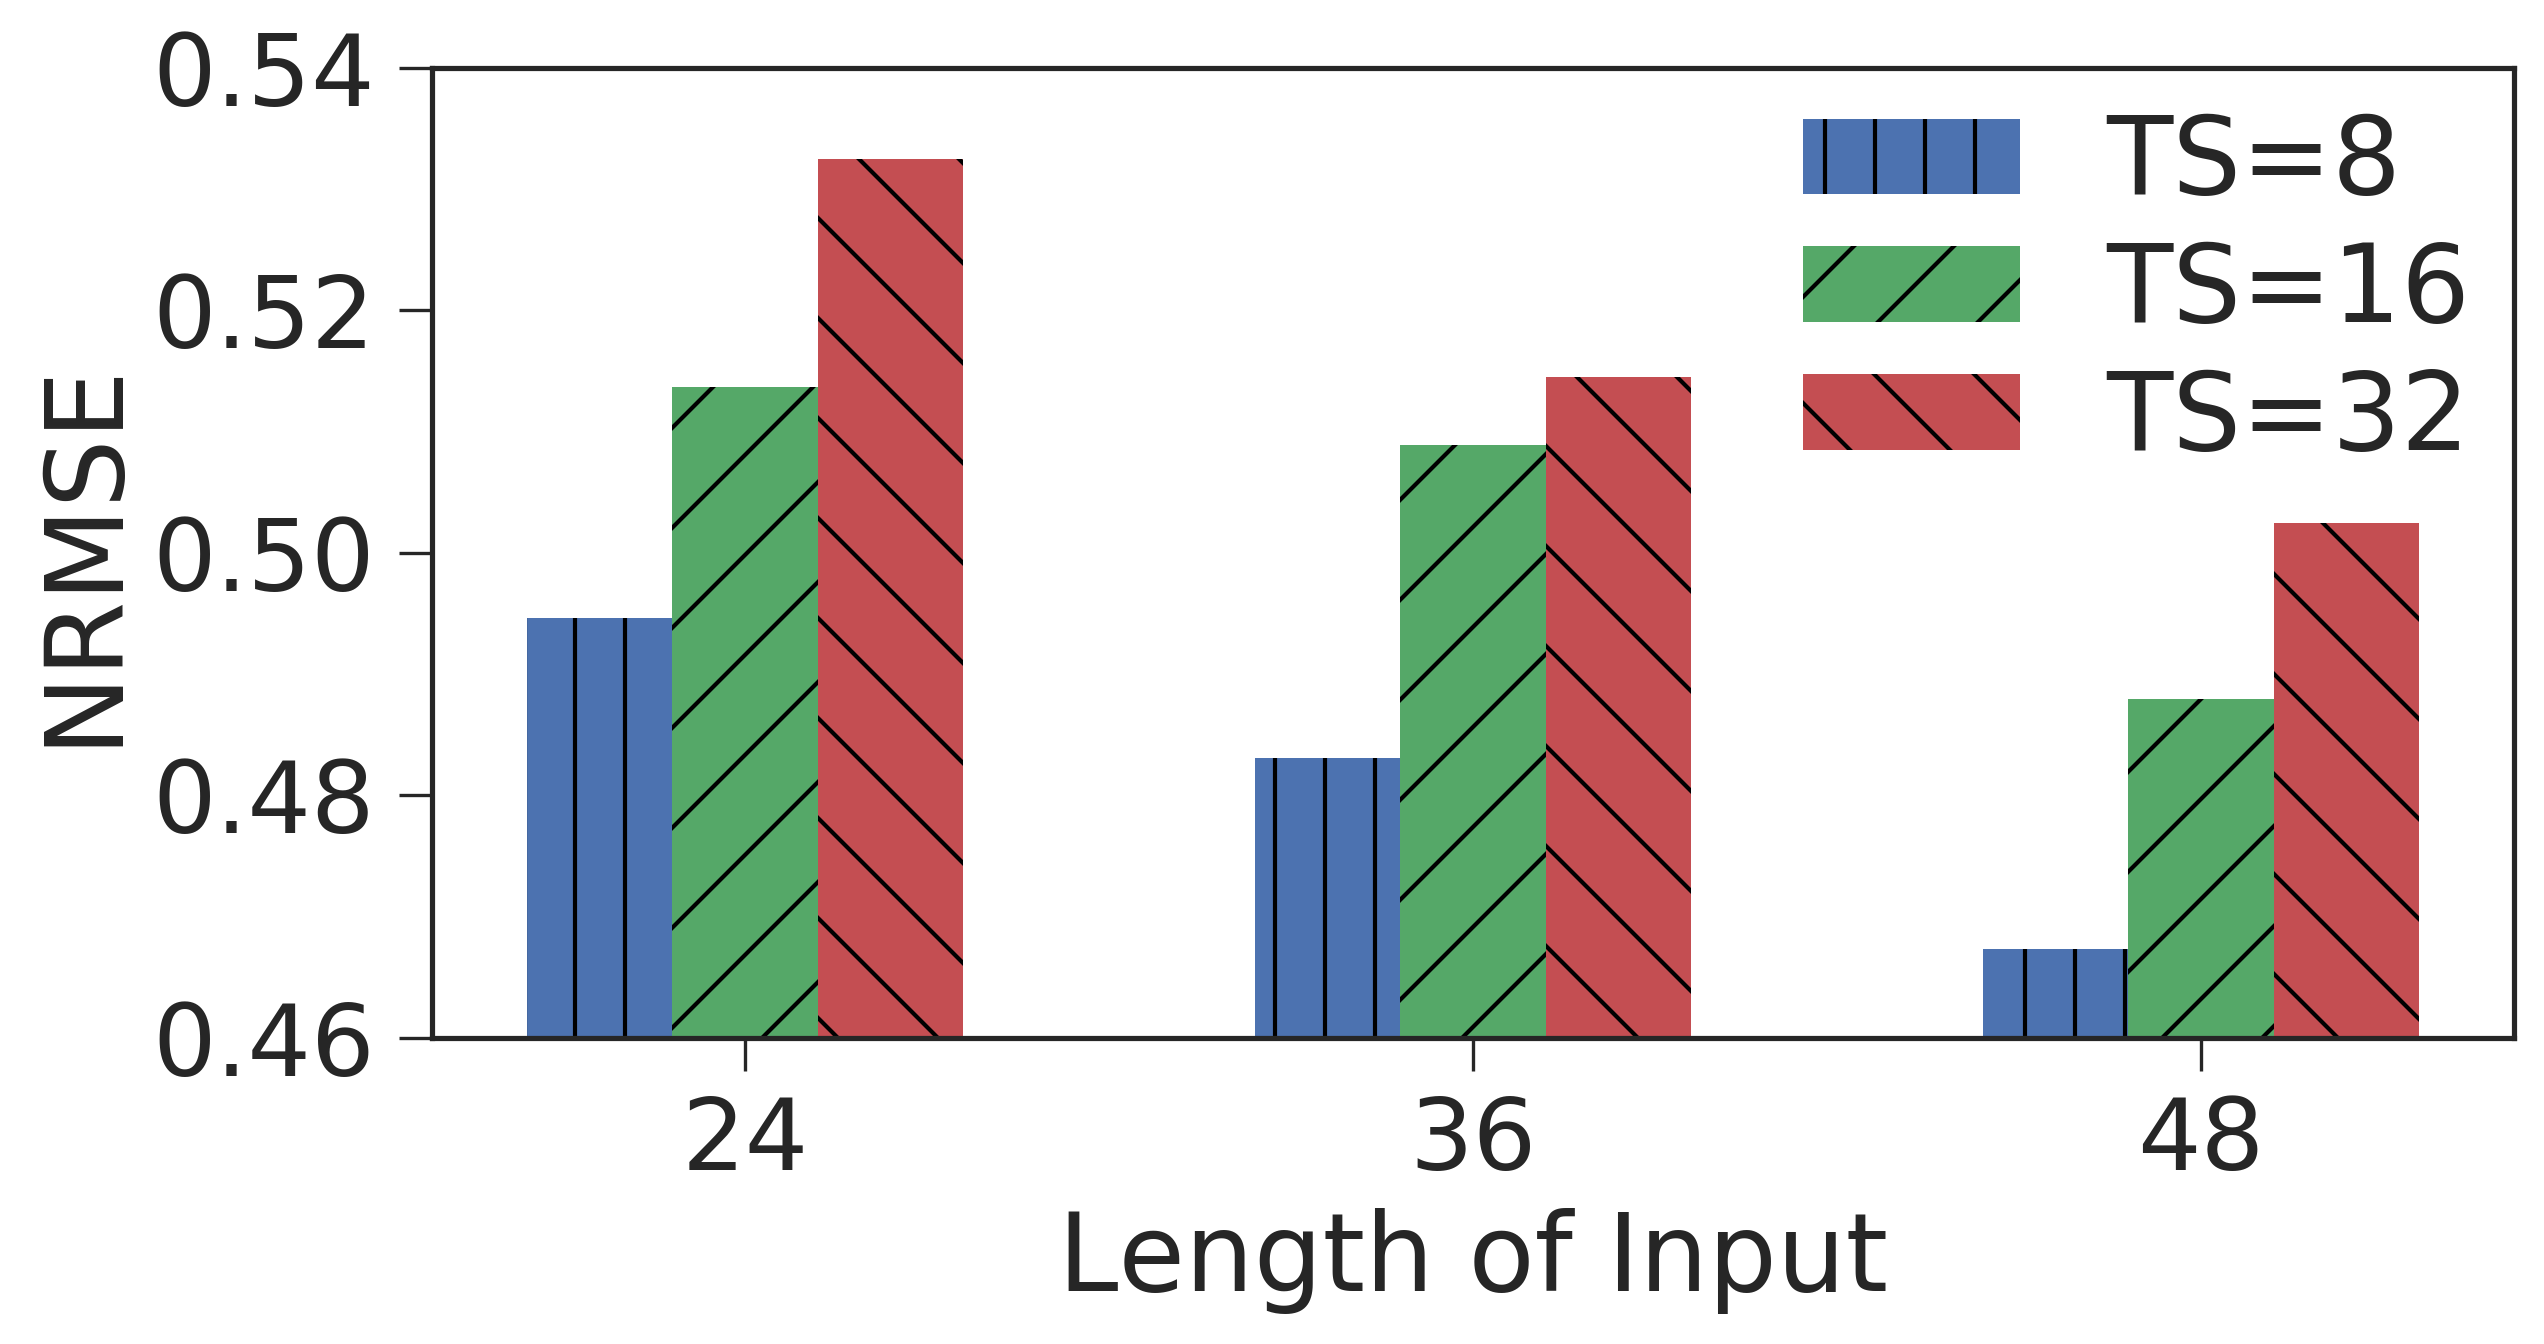}}\\
    \subfigure[$\times2$ performance in CITY3.]{
        \includegraphics*[width=0.22\textwidth]{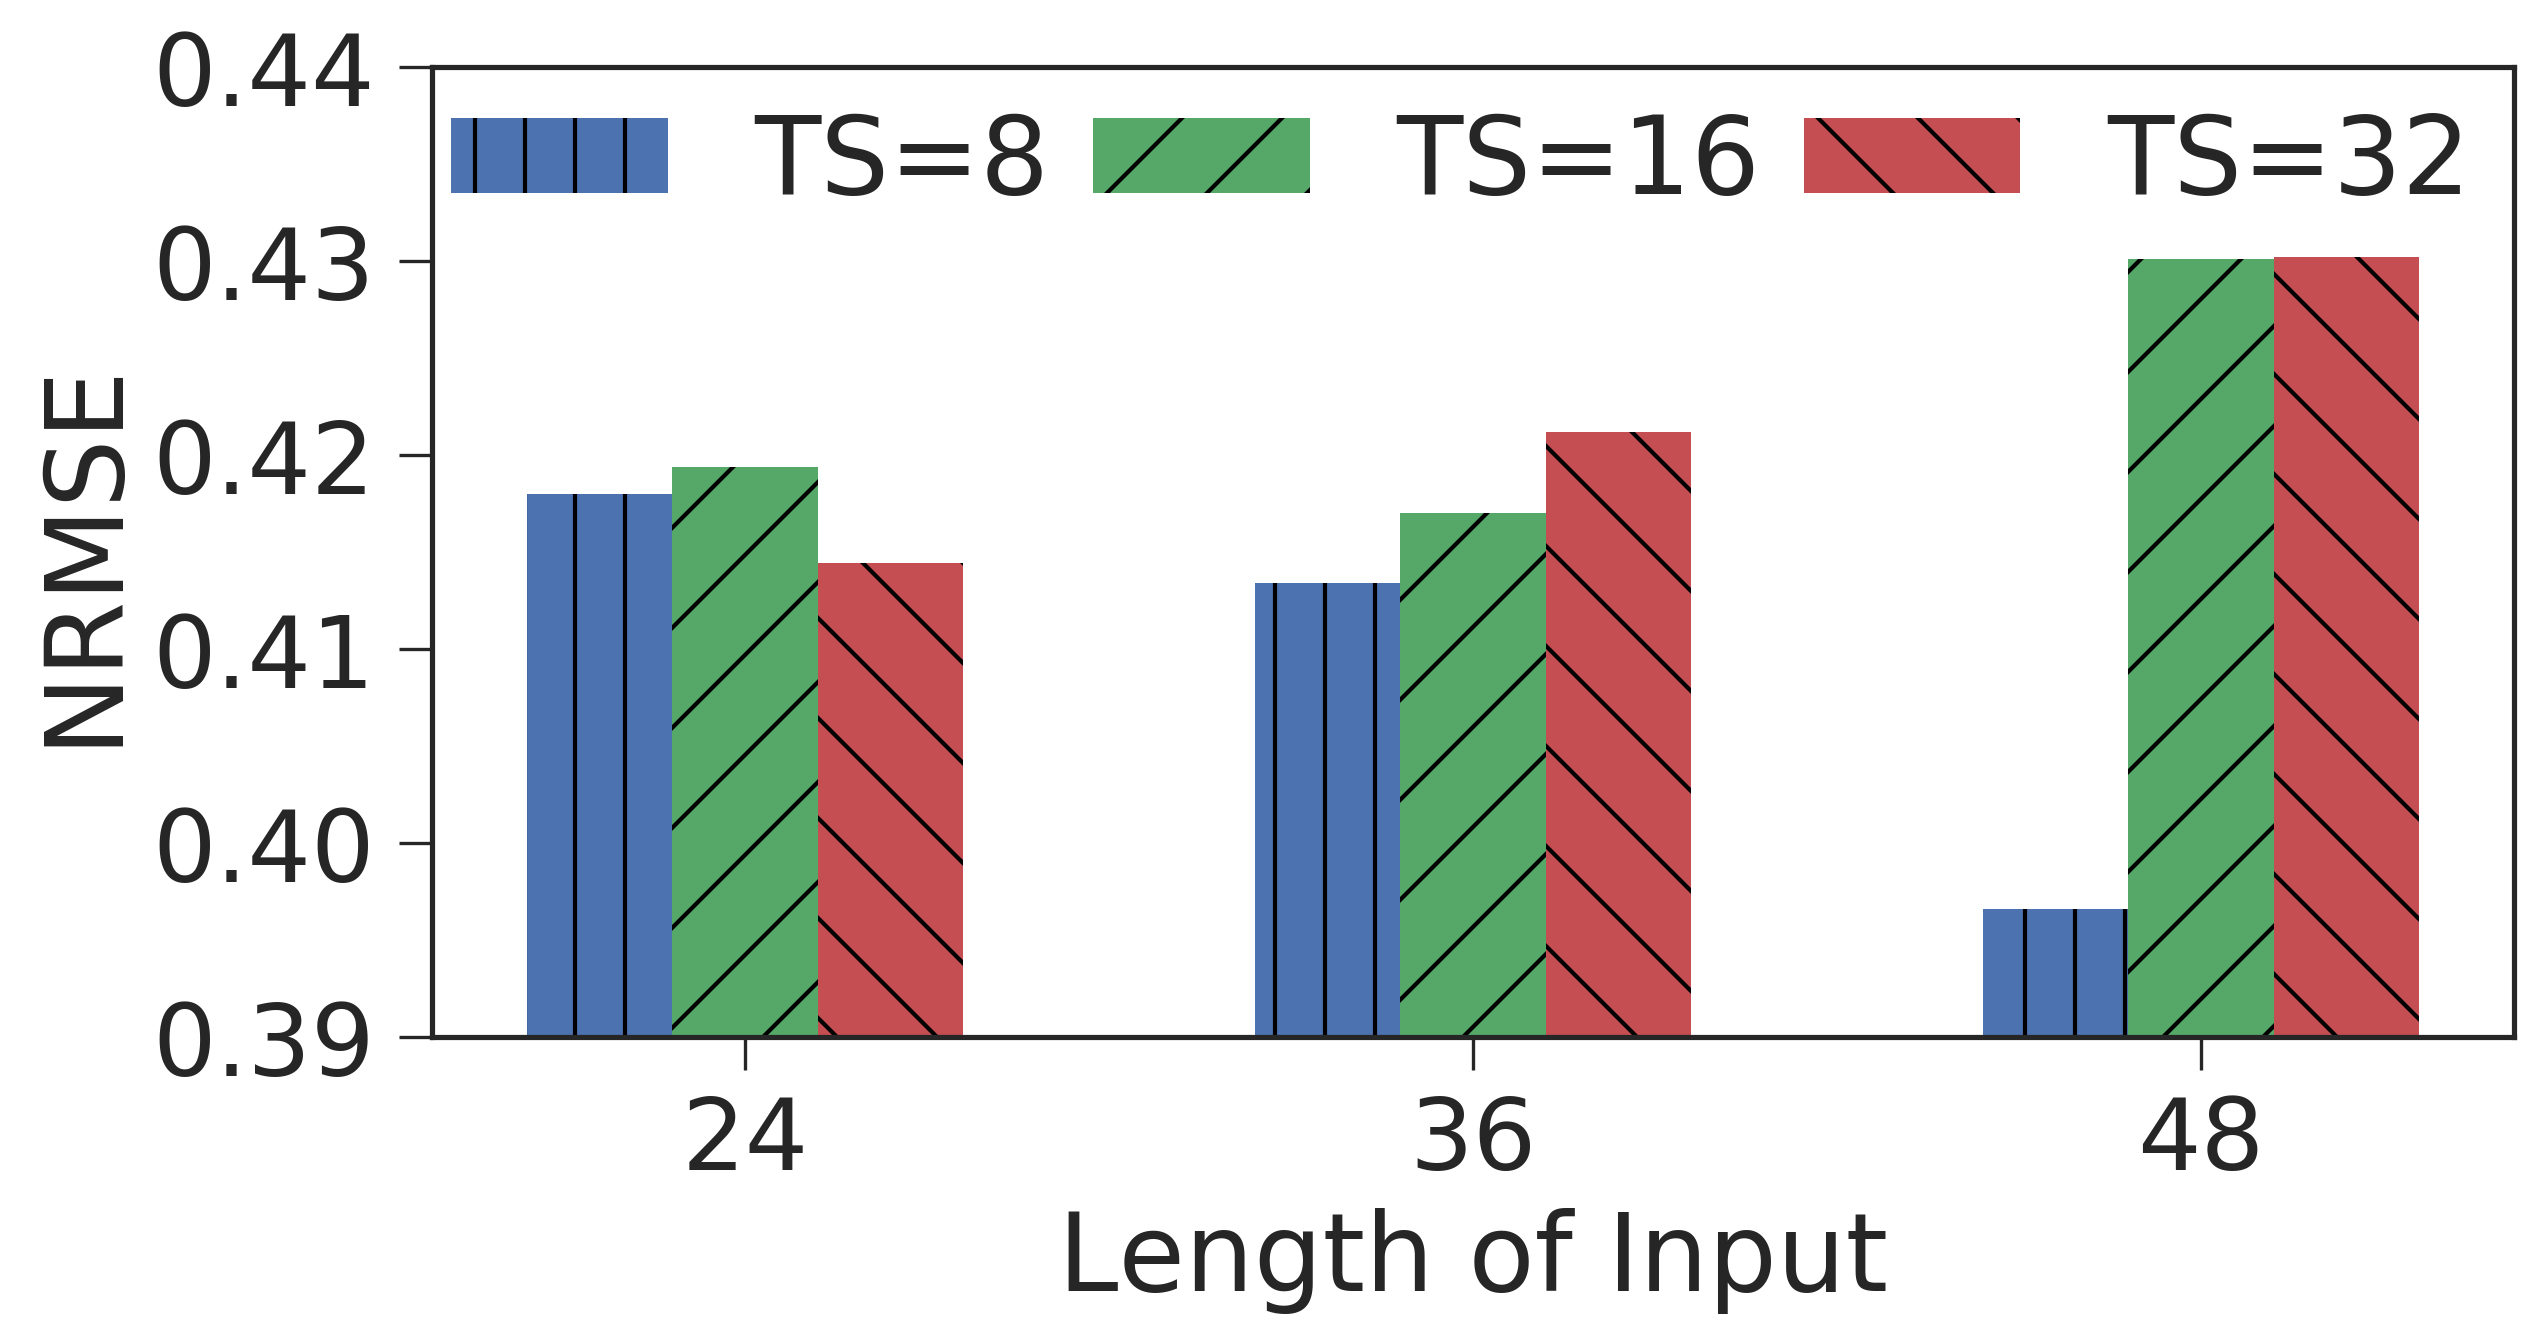}}
    \subfigure[$\times4$ performance in CITY3.]{
        \includegraphics*[width=0.22\textwidth]{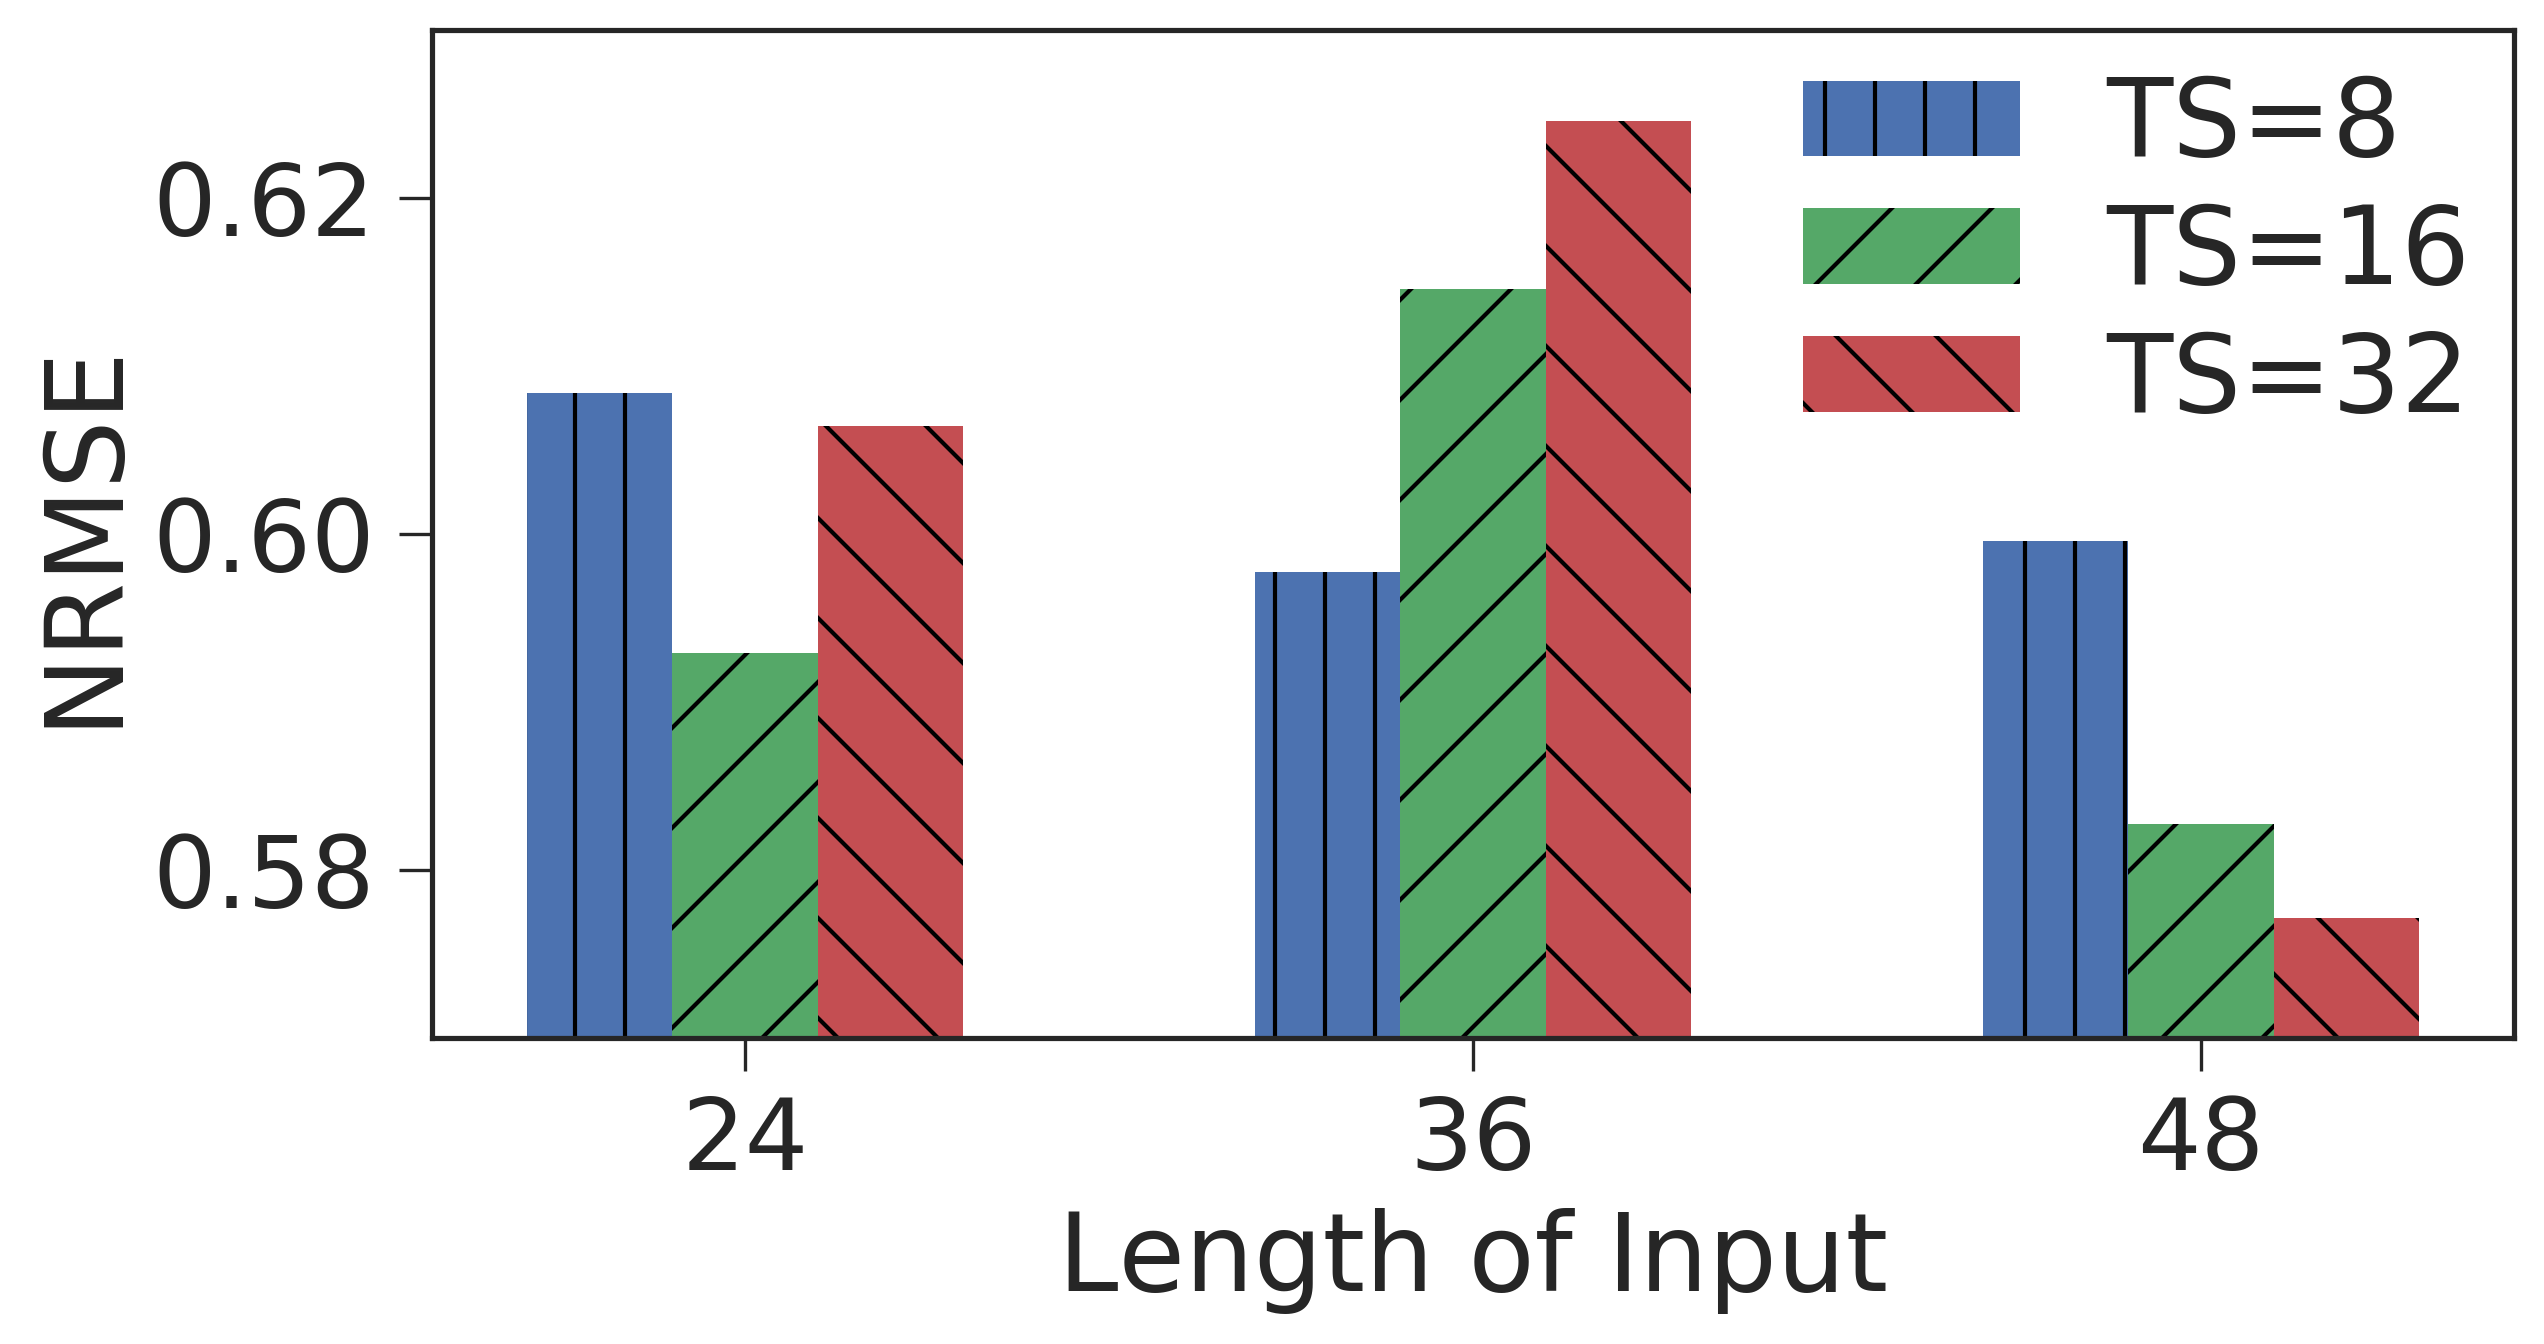}}
        \vspace{-0.2cm}
    \caption{The performance of \PSRNet with different lengths of input coarse-grained population maps (L) and time stride (TS).}
    \vspace{-0.4cm}
    \label{fig:frame_stride}
\end{figure}

%In these experiments, we employ fine-grained reference map to represent the satellite nightlight data, which is not an especially chosen time slot and nearby time slots have similar effect with it.
\begin{figure}[htbp]

    \subfigure[$\times2$ performance in CITY2.]{
        \includegraphics*[width=0.22\textwidth]{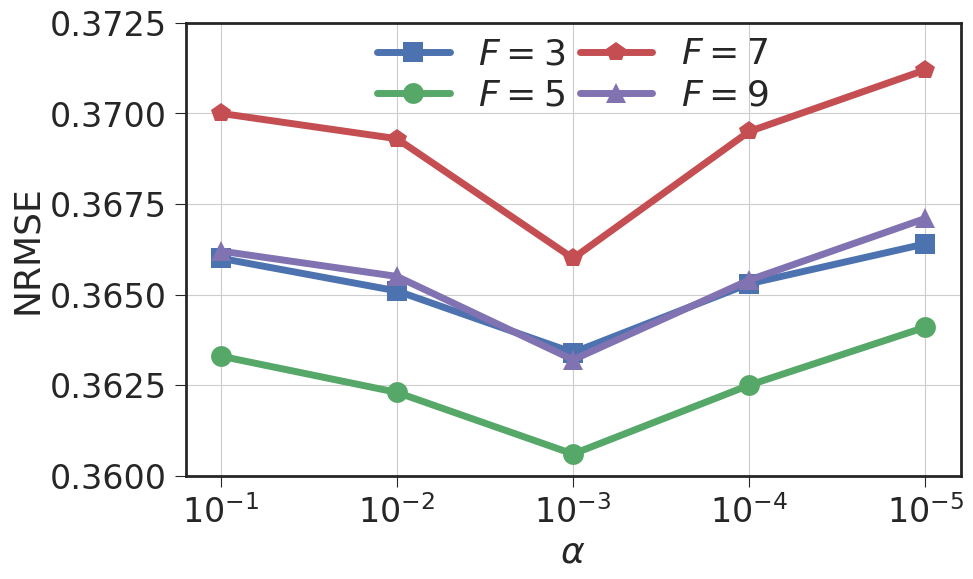}}
    \subfigure[$\times4$ performance in CITY2.]{
        \includegraphics*[width=0.22\textwidth]{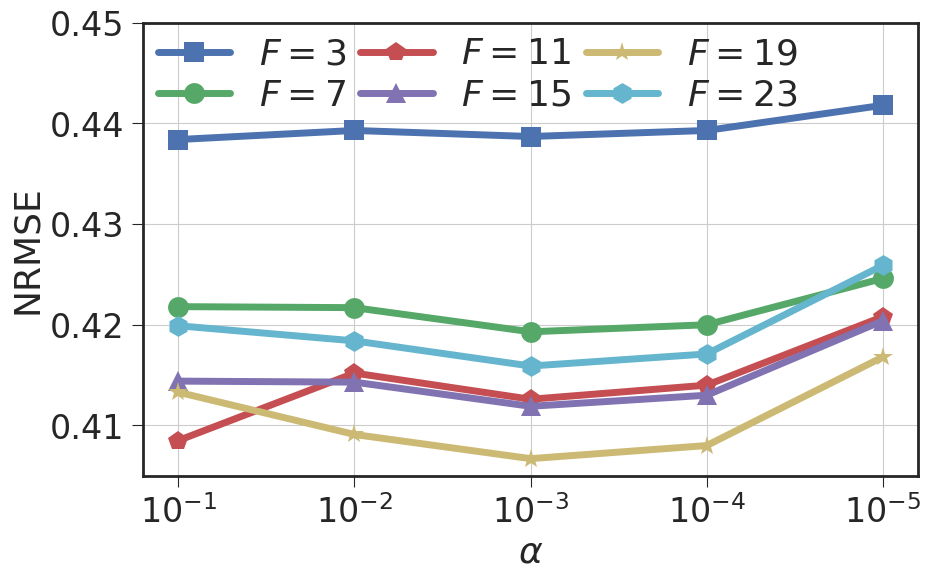}}\\
    \subfigure[$\times2$ performance in CITY3.]{
        \includegraphics*[width=0.22\textwidth]{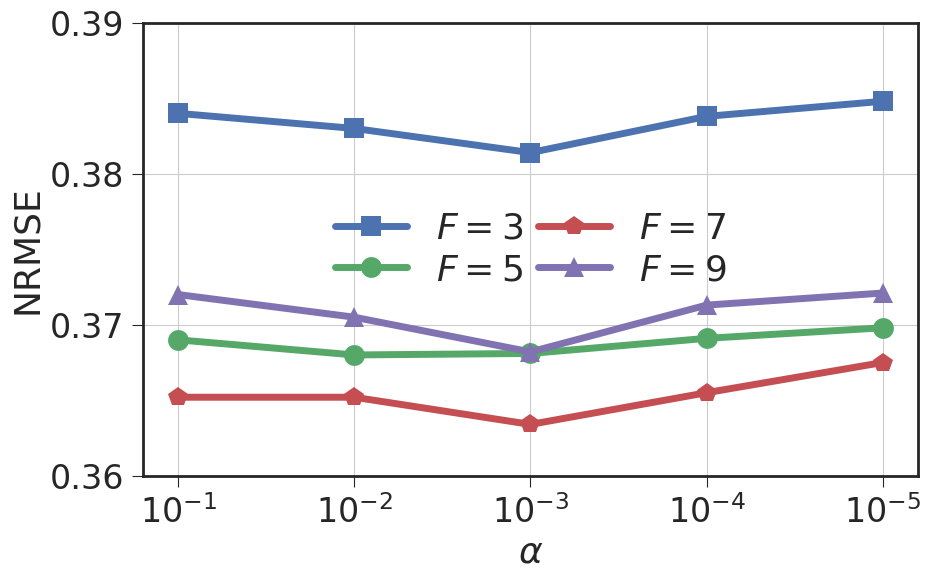}}
    \subfigure[$\times4$ performance in CITY3.]{
        \includegraphics*[width=0.22\textwidth]{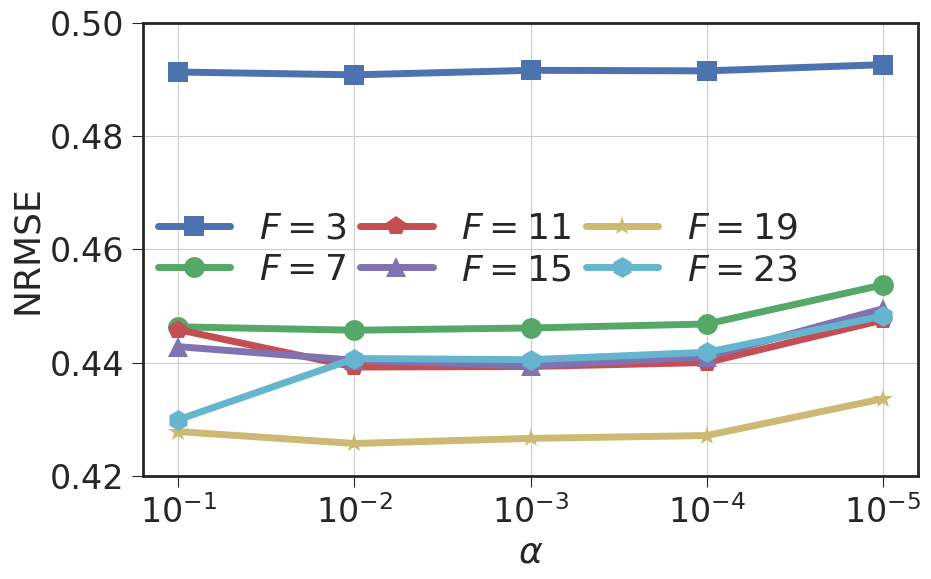}}
     \vspace{-0.2cm}
    \caption{The performance of \PSRNet with different number of generated fine-grained population map (F) and different $\alpha$ in the loss function of \PGNetns.}
    \label{fig:GAN_parameters}
    \vspace{-0.4cm}
\end{figure}

\subsubsection{Hyper-parameters Study of \emph{\PGNetns}}
For \PGNetns, we do a series of experiments about two hyper-parameters: the number of augmented fine-grained maps (F) and the weight of loss function $\alpha$, whose results are shown in Figure~\ref{fig:GAN_parameters}. Firstly, according to section~\ref{sec:Method}, both of the prediction loss $L_{MSE}$ and the classification loss $L_{C}$ are employed in our loss function $L = L_{C} + \alpha L_{MSE}$, while $\alpha$ is used to balance these two losses. Note that in the pre-training of \PGNetns, $L_{C}$ is usually between $0.1$ and $1$, whereas $L_{MSE}$ is usually between $150$ and $500$. For most curves in these sub-figures, \PSRNet shows the best performance when $\alpha = 10^{-3}$ or $10^{-4}$. In these spans of $\alpha$, $L_{C}$ and $\alpha L_{MSE}$ have similar values. That shows both $L_{C}$ and $L_{MSE}$ are effective for our model, and when these two losses are balanced, \PSRNet will have better performance.

Moreover, the experiment about the impact of the number of augmented fine-grained population distribution maps (F) shows another trade-off in \PGNetns, that is, the trade-off between the diversity and the quality of synthetic data. Results are presented in Figure~\ref{fig:GAN_parameters}. We employ category-aware POI density map to generate fine-grained population flows in target cities and then use these flow maps with the referenced fine-grained population distribution to obtain the final dynamic fine-grained population distribution. During this procedure, the quality of the augmented fine-grained population distribution map becomes worse as the time slot becomes further to the time of the reference map because the error of the synthetic data is accumulated. Therefore, although more augmented population maps could enrich data for training, they also damage the quality of fine-tuning. Besides, we find that \PSRNet is especially effective in high up-scaling scenarios. Compared with $\times2$ task, less spatial-temporal information are provided by coarse-grained maps in $\times4$ task. Thus, the generated maps from \PGNet contains more relative information and help more for the population mapping.

\subsubsection{Complexity Analysis}
To compare the complexity of \PSRNet and baselines, we present the memory-usage of each model and its RMSE in the $\times2$ task in CITY2, which is presented in Figure~\ref{fig:memory}. In Figure~\ref{fig:memory}, models on the left side have less memory usage and models in the downside have better performance of population mapping. We can find that the models RBPN and DBPN, have the highest memory usage while they have similar RMSE with RRN and RCAN. Moreover, since UrbanFM is specially designed for urban scenario, it obtain the state-of-the-art performance in all baselines. DeepDPM is a light-weight model so it has the least memory usage. Compare with these model, our \PSRNet is more effective to capture the spatial-temporal knowledge of sequential population maps with similar memory usage.

\begin{figure}[htb]
\vspace{-0.3cm}
\centering
\includegraphics[width=0.35\textwidth]{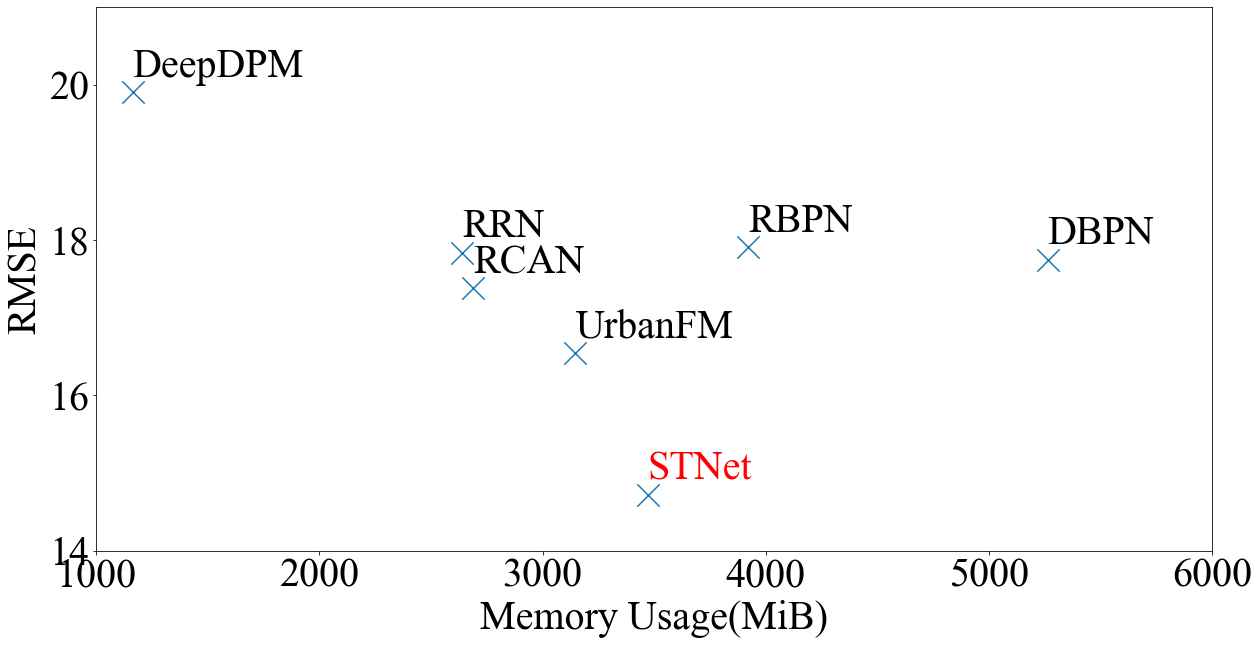}
\vspace{-0.2cm}
\caption{The memory usage and performance of \PSRNet and baselines of $\times2$ task in CITY2.}
\label{fig:memory}
\vspace{-0.4cm}
\end{figure}

\subsection{Complete Experiments' Results}
In addition to the results in Evaluation Section~\ref{sec:Exp}, in which only $3$ metrics, $\times 2$ task, and $\times 4$ task are included. We represent the complete table of all $5$ metrics and population mapping of all granularities ($\times 2$, $\times 4$, and $\times 8$) in Table~\ref{table:complete}. The experiments of cross-cities secnario and the comparison of different variants in Ablation Study are summarized in the left $3$ column. The complete results of cross-granularities scenario is summarized in the rightest column.
